# Supplementary material for: QAOAKit: A Toolkit for Reproducible Study, Application, and Verification of the QAOA
Source: arXiv:2110.05555 source file (2021-11-03)
Supplement: Supplementary file 1 [file appendix.tex]

\subsection{For authors}

Paper-Submission Deadline: \textbf{Friday, August 27, 2021}

Author Notification: Friday, October 8, 2021

``Authors are invited to submit original extended 2-page abstracts. The deadline is Friday, August 27, 2021.  Accepted papers will be able to submit a full paper for the workshop proceedings to be published in the IEEE Digital Library.

Full papers for the workshop proceedings will be due October 15, and must be at least 6 pages long, not including references and the reproducibility appendix. All submissions should be formatted according to the IEEE Conference Proceedings format (see https://www.ieee.org/conferences/publishing/templates.html).

Papers must be submitted electronically via Linklings on the Supercomputing website. 
Here are the instructions:

Log in to https://submissions.supercomputing.org/ and choose the "SC21 Workshop: Quantum Computing Software".

Full papers are expected to be published in the IEEE Xplore digital archive in collaboration with IEEE TCHPC.''

Updated deadlines:

Extended 2-page Abstract Submission Deadline:  Friday, August 27, 2021

Acceptance Notification: Friday, September 3, 2021

Camera-ready Manuscripts Due:  Friday, October 15, 2021

Workshop: Monday, November 15, 2021

Submission guidelines: \url{https://events.cels.anl.gov/event/27/page/64-paper-submission-guidelines}

\rs{Program committee member says: drop benchmarking, focus on standard format, on reproducibility and on being open to contributions as a public database.}

\subsubsection{What is the functionality that is missing?}

\rs{TODO @Ruslan: what is the standard format to aid parameter adding?}

\subsection{Listings}

An example of using \qaoakit{} to generate a QAOA circuit with optimal parameters is presented in Listing~\ref{lst:get_opt_params}.

\begin{lstlisting}[language=Python, caption={Using QAOAKit to generate and run a QAOA circuit with optimal parameters}, label={lst:get_opt_params}]
# build graph
import networkx as nx 
G = nx.star_graph(5)
# grab optimal angles
from QAOAKit import opt_angles_for_graph, angles_to_qaoa_format
p = 3
angles = angles_to_qaoa_format(
    opt_angles_for_graph(G,p))
# build circuit and print measurement outcomes
from QAOAKit.qaoa import get_maxcut_qaoa_circuit
qc = get_maxcut_qaoa_circuit(
    G, angles['beta'], angles['gamma'])
qc.measure_all()
# run circuit
from qiskit.providers.aer import AerSimulator
backend = AerSimulator()
print(backend.run(qc).result().get_counts())
\end{lstlisting}

Transferability figure:
